# Supplementary material for: Enhanced zero-bias conductance peak and splitting at mesoscopic interfaces between an $s$-wave superconductor and a 3D Dirac semimetal
Source: arXiv:1612.09064 source file (2016-12-29)
Supplement: Supplementary file 1 [file Cd3As2_Nb_supplementary.pdf]

# Enhanced zero-bias conductance peak and splitting at mesoscopic interfaces between an $s$-wave superconductor and a 3D Dirac semimetal

Leena Aggarwal[1], Sirshendu Gayen[1], Shekhar Das[1], Gohil S. Thakur[2], Ashok K. Ganguli[2,3] & Goutam Sheet[1]

[1]*Department of Physical Sciences, Indian Institute of Science Education and Research(IISER), Mohali, Sector 81, S. A. S. Nagar, Manauli, PO: 140306, India.*

[2]*Department of Chemistry, Indian Institute of Technology, New Delhi 110016, India.*

[3]*Institute of Nano Science & Technology, Mohali 160064, India.*

## Material Synthesis and characterization

All the details related to material characterization has mentioned in the supplementary report of reference [1][1].

## Low-temperature measurements

The low temperature measurements were performed in a liquid helium cryostat working down to 1.4 K. The cryostat is equipped with a dynamic variable temperature insert (VTI) inside which there is one static VTI. The bottom part of the static VTI is made of copper for efficient cooling. The sample goes inside the static VTI which is first evacuated and then filled with dry helium exchange gas. The cryostat is also equipped with a three-axis vector magnet. The vector magnet can apply a maximum magnetic field of 6 T along the vertical direction using a superconducting solenoid and 1T in the horizontal plane using four superconducting Helmholtz coils. For the measurements presented in this paper, magnetic field was applied in the vertical direction, perpendicular to the sample surface using the solenoid.

**Point-contact Spectroscopy:** Point-contact spectroscopy experiments were performed using a home-built low-temperature probe. The probe consists of a long stainless steel tube at the end of which the probe-head is mounted. The probe head is equipped with a 100 threads per inch (*t.p.i.*) differential screw that is rotated by a shaft running to the top of the cryostat. The screw drives a tip-holder up and down with respect to the sample. The sample-holder is made of a 1" dia. copper disk. A cernox thermometer was mounted on the copper disc for the measurement of the temperature. The temperature of the disc was varied by a heater mounted on the same copper disc. The tips were fabricated by cutting a 0.25 mm dia. metal wire at an angle. The tip was mounted on the tip holder and two gold contact leads were made on the tip with silver epoxy. The samples were mounted on the sample holder and two silver-epoxy contact leads were mounted on the sample as well. These four leads were used to measure the differential resistance ($dV/dI$) across the point-contacts. The leads 3 and 4 were used to carry out the two-probe resistivity measurements.

The point-contact spectra were captured by ac-modulation technique using a lock-in-amplifier (Model: SR830 DSP) (as shown in the schematic diagram) with automated data acquisition software (LabView). A voltage to current converter was fabricated to which a dc input coupled with a very small ac input was fed. The output current had a dc and a small ac component. This current passed through the point-contact. The dc output voltage across the point-contact, $V$ was

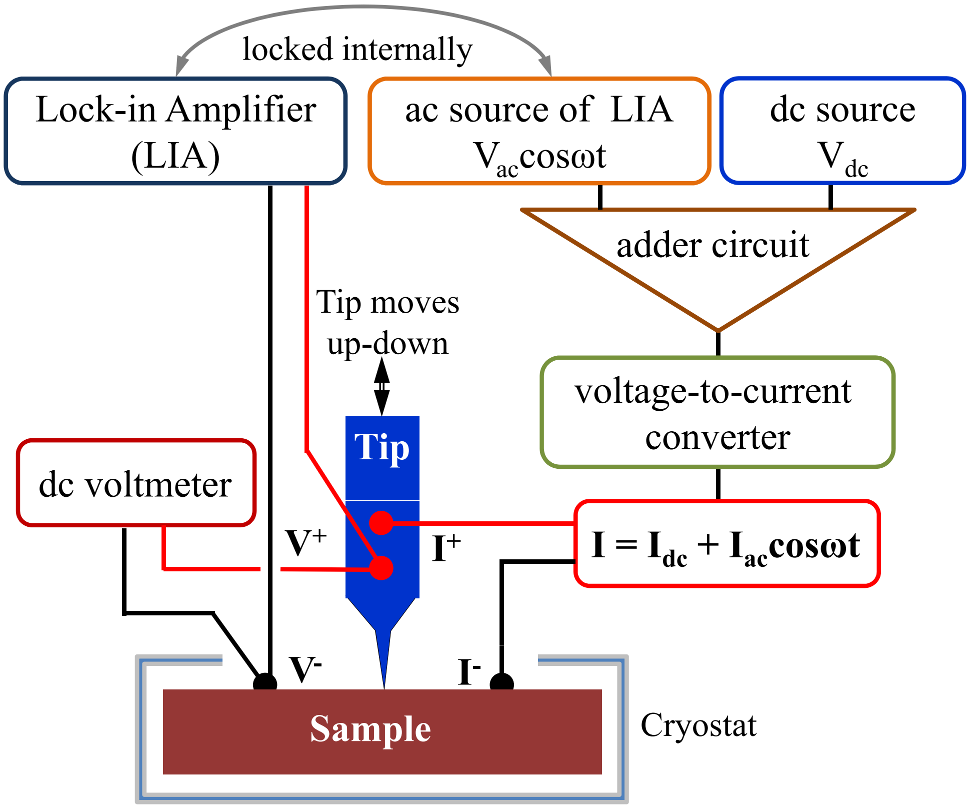


**Fig. S1:** Schematic diagram describing the point-contact spectroscopy measurements.

measured by a digital multimeter (model: Keithley 2000 ) and the ac output voltage, locked at first harmonic (for this measurement $f = 670\,\mathrm{Hz}$), was measured by the lock-in-amplifier. The ac voltage is proportional to $dV/dI$ and inverse of which with proper normalization is plotted against $V$ to obtain the point-contact spectrum.

**Different transport regimes of point-contact spectroscopy:**

The resistance $R_{PC}$ of such a point contact is given by Wexlers formula[2]: $R_{PC} = \frac{2h/e^2}{(ak_F)^2} + \Gamma(l/a)\frac{\rho(T)}{2a}$, where $h$ is Planck's constant, $e$ is the charge of a single electron, $a$ is the contact diameter, $\Gamma(l/a)$ is a slowly varying function of the order of unity, $\rho$ is the bulk resistivity of the material and $T$ is the effective temperature at the point contact. The first term is known as the ballistic or Sharvin resistance[3] ($R_S$) and is independent of the bulk resistivity of the materials forming the point contact.

The second term is called the Maxwell resistance ($R_M$), which depends directly on the resistivity of the materials. The above equation also suggests that when the contact diameter is small compared to electronic mean free path (ballistic regime) then $R_S$ dominates, and when the con-

tact diameter is large (thermal regime) then $R_M$ contributes most to the total contact resistance. Therefore resistive transitions lead to non linearities in the $I-V$ characteristics, corresponding to $R_M$ of point contacts[4]. No spectroscopy can be performed in the thermal regime owing to the permitted inelastic processes at the interface. The observation of two sharp peaks symmetric about $V = 0$ in the $dV/dI$ versus $V$ plots obtained from non-ballistic point contacts is a known signature of superconductivity[4,5]. The peaks appear when the dc current flowing through the point contact reaches the critical current for the given point contact[4].

**Superconducting energy gap from ballistic data:** The symmetric peaks about $V = 0$ in the ballistic regime data (for example, refer to Figure 1(b)) of $dI/dV$ versus $V$ roughly correspond to the superconducting gap voltage $\pm\Delta/e$. However, the Andreev-reflection-driven peaks in the ballistic regime spectra are significantly broader than what is expected from the BTK theory that is traditionally used to analyse Andreev reflection spectra obtained on conventional BCS (Bardeen, Cooper, Schrieffer) superconductors[6]. This might be due to a large inelastic broadening[7,8] parameter at the interface and an unconventional pairing. To analyse such spectra quantitatively a theoretical model for Andreev reflection taking into account the non-trivial topological properties of one of the electrodes forming the point contact must be developed. The peak positions thus obtained give an approximate but reasonable estimate of the gap amplitude.

## Some additional data

Figure S2 shows the addition data for Nb/$Cd_3As_2$ point-contact of spectrum type-II for different point-contact. The spectra show the splitting of the ZBCP with systematic evolution with increasing magnetic field and disappearance beyond 6 T. Figure S3 shows the full set of magnetic field dependent spectra for the same point-contact as shown in figure 2(d) of spectrum type-II.

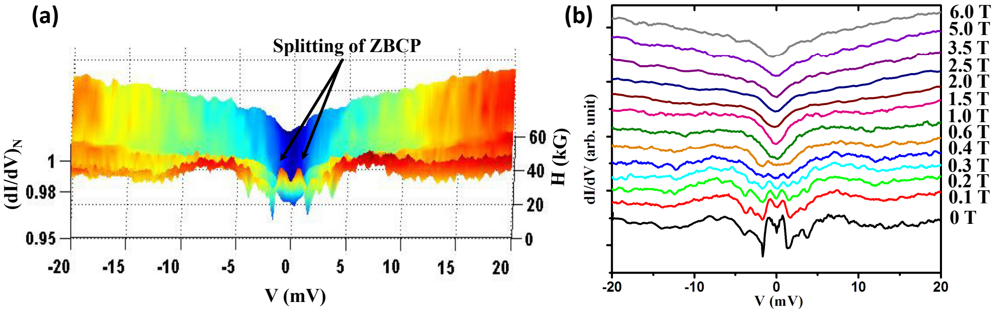


**Fig. S2:** (a) 3-D magnetic field dependent spectra for Nb/$Cd_3As_2$ point-contact of spectrum type-II showing the splitting of ZBCP for another point contact. (b) Corresponding 2D data.

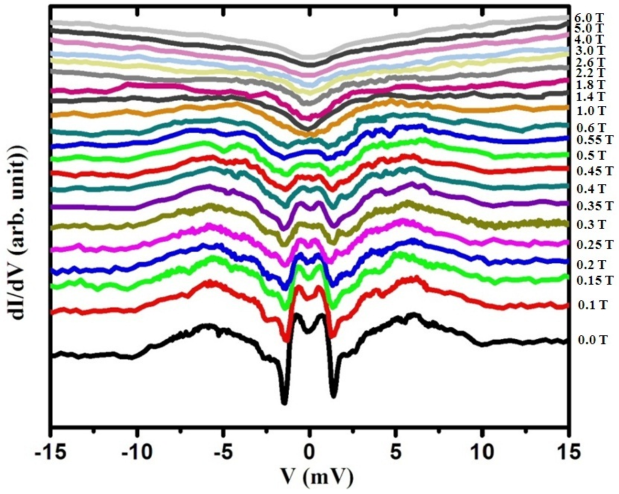


**Fig. S3:** Full set of field dependent spectra for Figure 2(d) in the main manuscript

1 Aggarwal, L., Gaurav, A., Thakur, G. S., Haque, Z., Ganguli, A. K. & Sheet, G. Unconventional superconductivity at mesoscopic point contacts on the 3D Dirac semimetal $Cd_3As_2$. *Nature Materials* **15**, 32 (2016).

2 Wexler, A. The size effect and the non-local Boltzmann transport equation in orifice and disk geometry. *Proc. Phys. Soc.* **89**, 927 (1966).

3 Datta, S. Electronic Transport in Mesoscopic Systems (Cambridge Univ. Press, 1995).

4 Sheet, G., Mukhopadhyay, S. & Raychaudhuri, P. Role of critical current on the point-contact Andreev reflection spectra between a normal metal and a superconductor. *Phys. Rev. B* **69**, 134507 (2004).

5 Naidyuk, Y. G. & Yanson, I. K. Point-contact Spectroscopy (Springer, 2004).

6 Blonder, G. E., Tinkham, M. & Klapwijk, T. M. Transition from metallic to tunneling regimes in superconducting microconstrictions: Excess current, charge imbalance, and supercurrent conversion. *Phys. Rev. B* **25**, 4515 (1982).

7 Sato, M., Tanaka, Y., Yada, K. & Yokoyama, T. Topology of Andreev bound states with flat dispersion. *Phys. Rev. B* **83**, 224511 (2011).

8 Plecenik, A., Grajcar, M., Beaka, S., Seidel, P. & Pfuch, A. Finite-quasiparticle-lifetime effects in the differential conductance of $Bi_2Sr_2CaCu_2O_y/Au$ junctions. *Phys. Rev. B* **49**, 10016 (1994).
